# Supplementary material for: AutoHete: An Automatic and Efficient Heterogeneous Training System for LLMs
Source: arXiv:2503.01890 source file (2025-02-27)

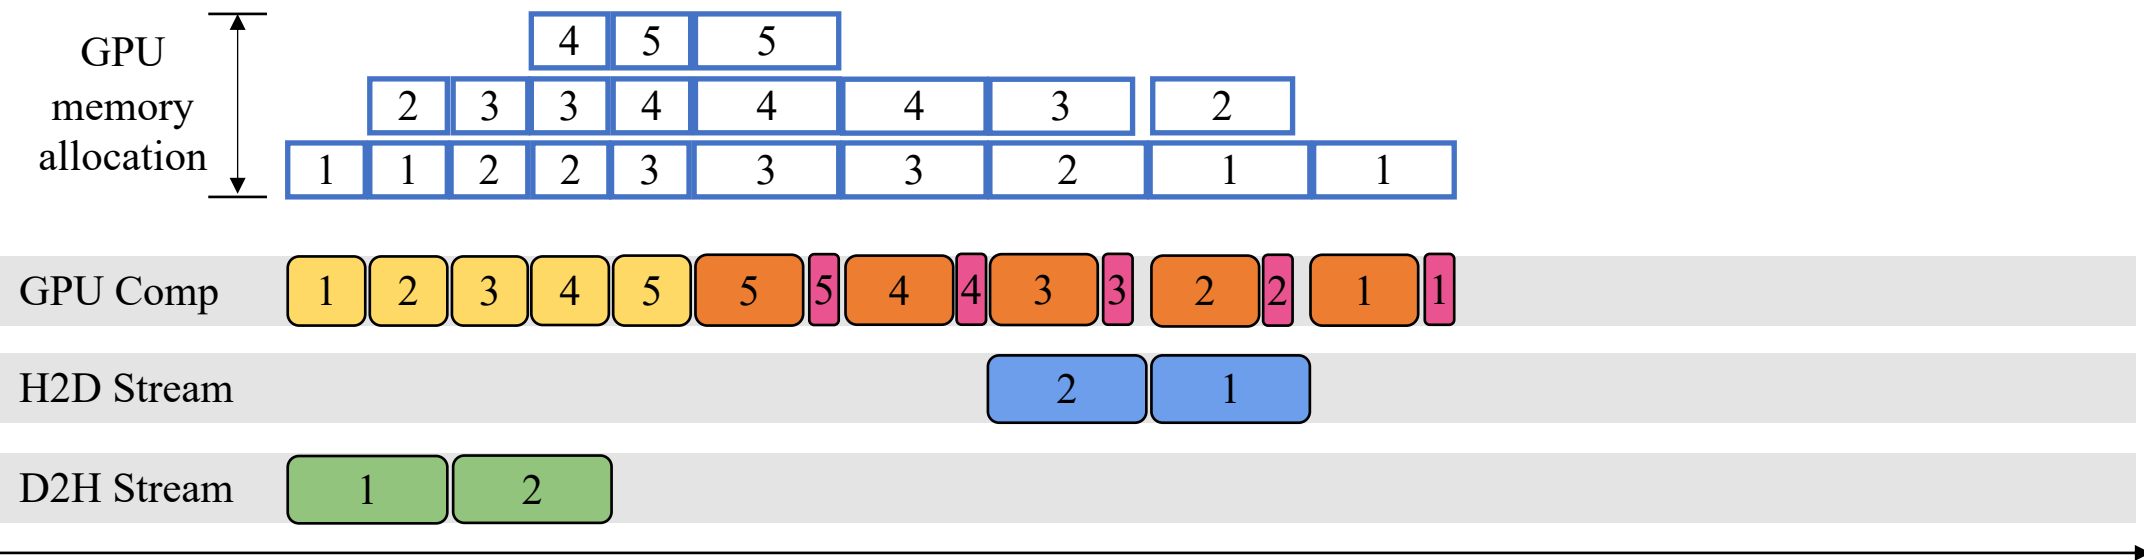

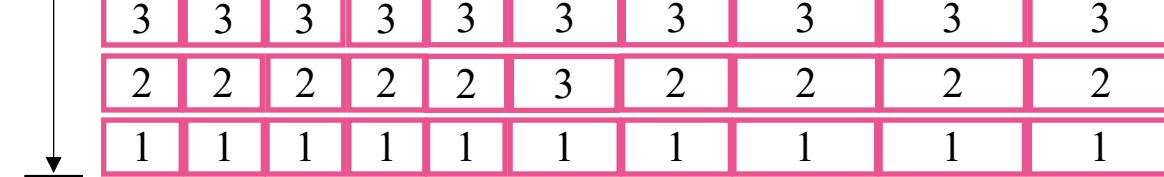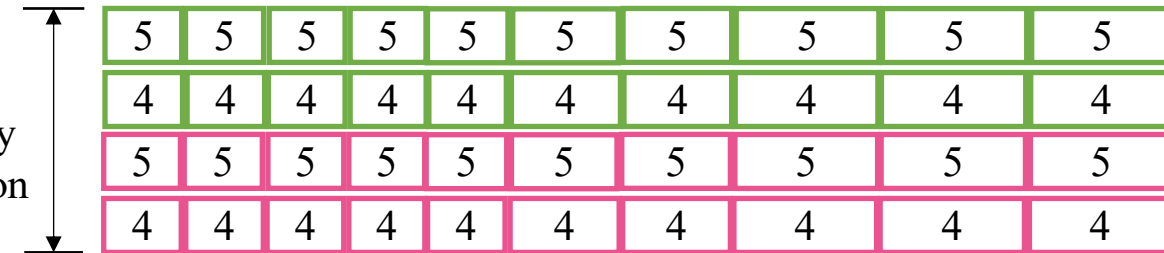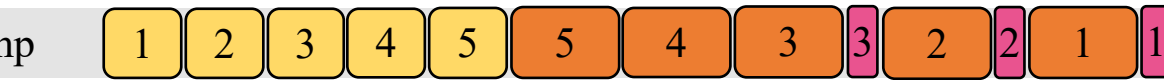

Supplement: Supplementary file 1 [file appendix_b.pdf]
